# Supplementary material for: Thermodynamic Bifurcations of Boiling in Solid-State Nanopores
Source: arXiv:2308.12597 ancillary file (2023-08-24)
Supplement: Supplementary file 1 [file Supplementary_Material.pdf]

# Supplemental Material for "Thermodynamic Bifurcations of Boiling in Solid-State Nanopores"

Soumyadeep Paul,[1,*] Yusuke Ito,[1] Wei-Lun Hsu,[1] and Hirofumi Daiguji[1,†]

[1]*Department of Mechanical Engineering, The University of Tokyo, 7-3-1, Hongo, Bunkyo-ku, Tokyo 113-8656, Japan*

## S1. SEM IMAGE OF A CYLINDRICAL NANOPORE

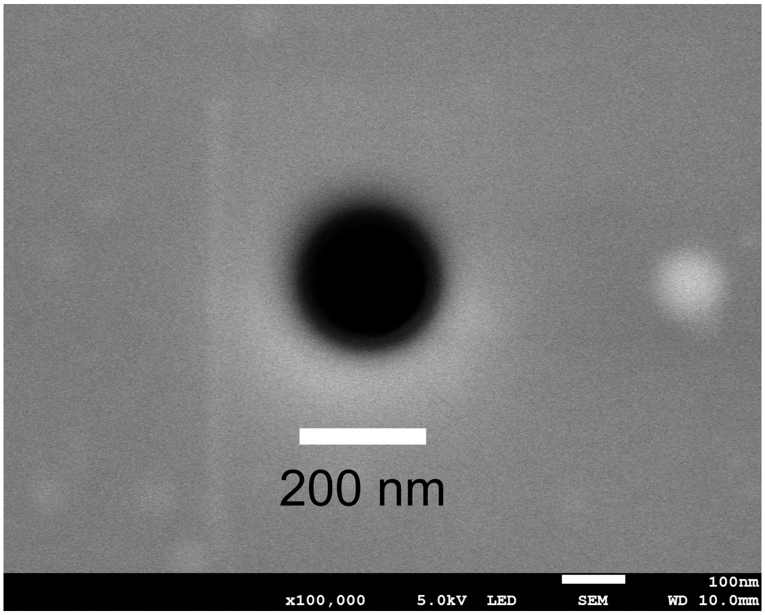


FIG. S1: SEM image of the 199 nm nanopore used in the present study.

## S2. CONTINUUM SIMULATIONS OF NANOPORE JOULE HEATING

We obtain the temperature distributions within the nanopore by performing numerical simulations, wherein we solve the energy-conservation equations in the liquid and the silicon nitride membrane:

$$\begin{aligned} &\frac{1}{y}\frac{\partial}{\partial y}\left(k_{\mathrm{w}} y \frac{\partial T}{\partial y}\right) + \frac{\partial}{\partial z}\left(k_{\mathrm{w}}\frac{\partial T}{\partial z}\right) + \sigma|\mathbf{E}|^2 = 0, \\ &\frac{1}{y}\frac{\partial}{\partial y}\left(k_{\mathrm{m}} y \frac{\partial T}{\partial y}\right) + \frac{\partial}{\partial z}\left(k_{\mathrm{m}}\frac{\partial T}{\partial z}\right) = 0. \end{aligned} \tag{S1}$$

The above equations are solved on an axisymmetric reference frame, keeping the origin at the center of the nanopore $(y, z) = (0, 0)$, where $y$ is the radial coordinate and $z$ is the axial coordinate. The boundary conditions for temperature $T$ and ionic flux $\mathbf{J}$ on the simulation boundaries and the silicon nitride surface are shown in Fig. S2 (left inset). The subscripts 'w' and 'm' denote the liquid side and silicon nitride side of the interface. The no flux boundary condition

* Corresponding author: soumyadeep.paul@thml.t.u-tokyo.ac.jp
† Corresponding author: daiguji@thml.t.u-tokyo.ac.jp

for ion transport is applied on the bubble surface as shown in Fig. S2 (left inset), while the heat transfer boundary conditions applied on the liquid–vapor interface of the bubble ($S_{\rm LV}$) and the solid–vapor interface of the bubble ($S_{\rm SV}$) are discussed in Eqs. (2)–(5) in the main article. Here, $k_{\rm w}$ is the temperature-dependent thermal conductivity of water [1], $\mathbf{E}$ is the electric field in the electrolyte, $k_{\rm m}$ is the thermal conductivity of the silicon nitride membrane, and $\sigma$ is the electrical conductivity of the 3M aqueous NaCl electrolyte, which varies nonlinearly with temperature, and was fitted by an empirical relation by Levine *et al.* [1]:

$$\sigma = mT - b - \frac{(T - T_{\rm ref})^{\eta}}{\beta}. \tag{S2}$$

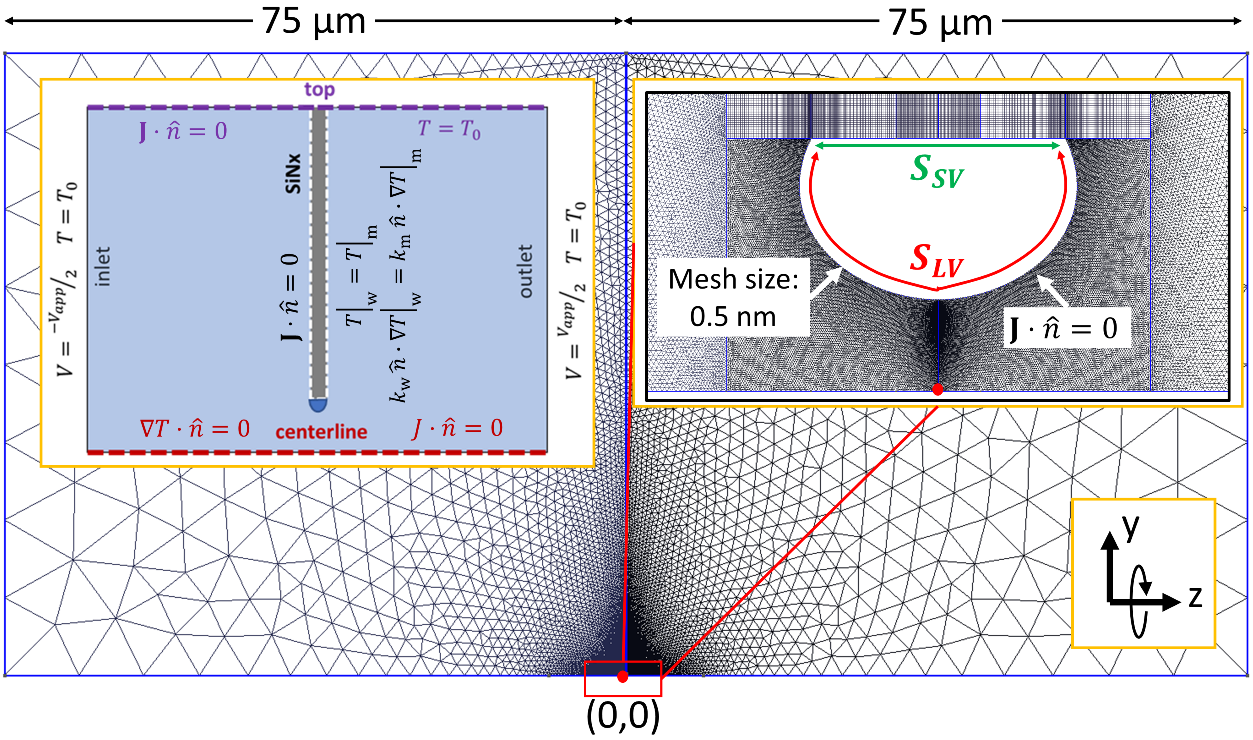


FIG. S2: Finite-volume mesh used for steady-state nanopore Joule heating simulations. The left inset shows the boundary conditions for temperature and ion flux, while the right inset shows a closeup of the mesh at the nanopore. A fine grid mesh of 0.5 nm is used on the bubble surface. $T_0 = 298.15$ K is the ambient temperature during experiments, which is applied as the far-field boundary condition at 75 µm away from the pore center. $\hat{n}$ is the surface normal unit vector pointing towards the solution.

Here, $m = 0.391\ \mathrm{S\,m^{-1}\,K^{-1}}$, $b = 0.391$ S/m, $\beta = 5.6 \times 10^4$, and $T_{\rm ref} = 293.15$ K. $\eta$ is the only parameter that is varied to fit the nanopore current during superheating. Levine *et al.* [1] used $\eta = 2.7$ to fit the Joule heating current for their 107 nm nanopore. Using a similar value of $\eta = 2.6$, we simulate all the boiling regimes for the 199 nm pore used in this current study. From the ion flux balance ($\nabla\cdot\mathbf{J} = 0$), we obtain the electric field inside the liquid:

$$\nabla\cdot(\sigma\nabla\phi) = 0. \tag{S3}$$

$\phi$ is the electric potential, and $\Delta\phi = V_{\rm app}$ is the voltage bias applied across the nanopore. $\mathbf{J} = \sigma\mathbf{E} = -\sigma\nabla\phi$ is the ionic flux. Due to the very thin electric double layers (Debye length $< 1$ nm) at the high salt concentration of 3M NaCl, the surface conductance has been neglected in comparison to the bulk conductance through the nanopore, having a diameter of 199 nm. However, due to the variation in electrical conductivity and permittivity with temperature, space charge densities are induced in the liquid which can be solved from Poisson's equation, $\rho_{\rm e} = \varepsilon_0\nabla\cdot\epsilon\mathbf{E}$. Here, $\varepsilon_0$, and $\epsilon$ are the dielectric permittivity of free space and temperature-dependent dielectric constant of water, respectively [1, 2]. According to our calculations as well as previous literature [1], the induced charge densities are minor [$\rho_{\rm e} \sim \mathcal{O}(10^4\ \mathrm{C/m^3})$], resulting in advective and diffusive currents which can be neglected in comparison to the conductive ionic flux, $\mathbf{J}$. Equations (S1)–(S3) are solved on a finite-volume mesh using the multiphysics software *arb* [3].

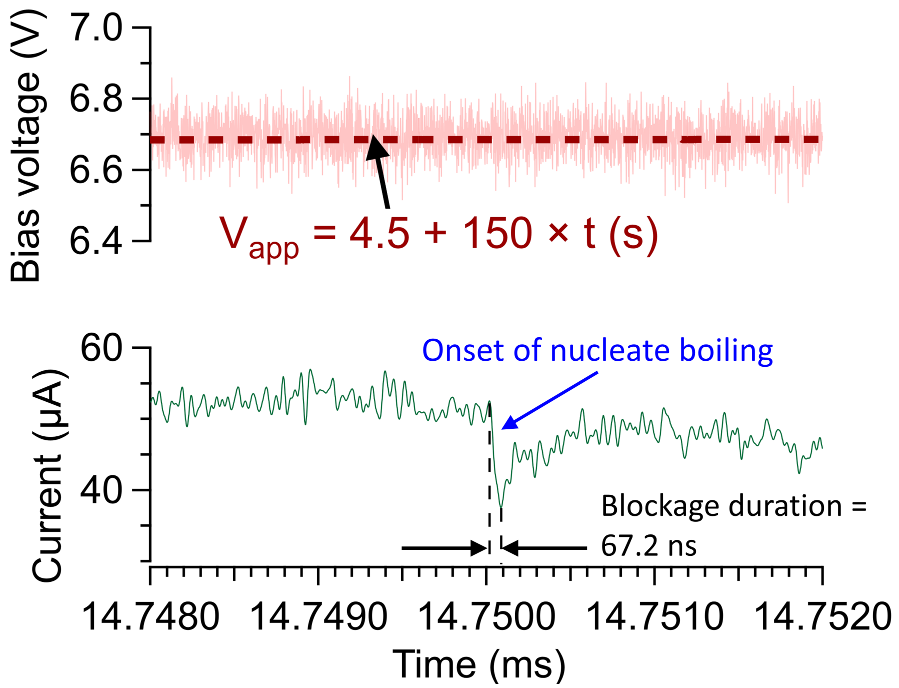


FIG. S3: First homogeneous bubble nucleation at 14.75 ms when the bias voltage is 6.7125 V and the steady-state pore center temperature reaches 562 K in each simulation. This value is close to the kinetic limit for homogeneous nucleation of 575 K [4]. The bubble blockage duration is 67.2 ns.

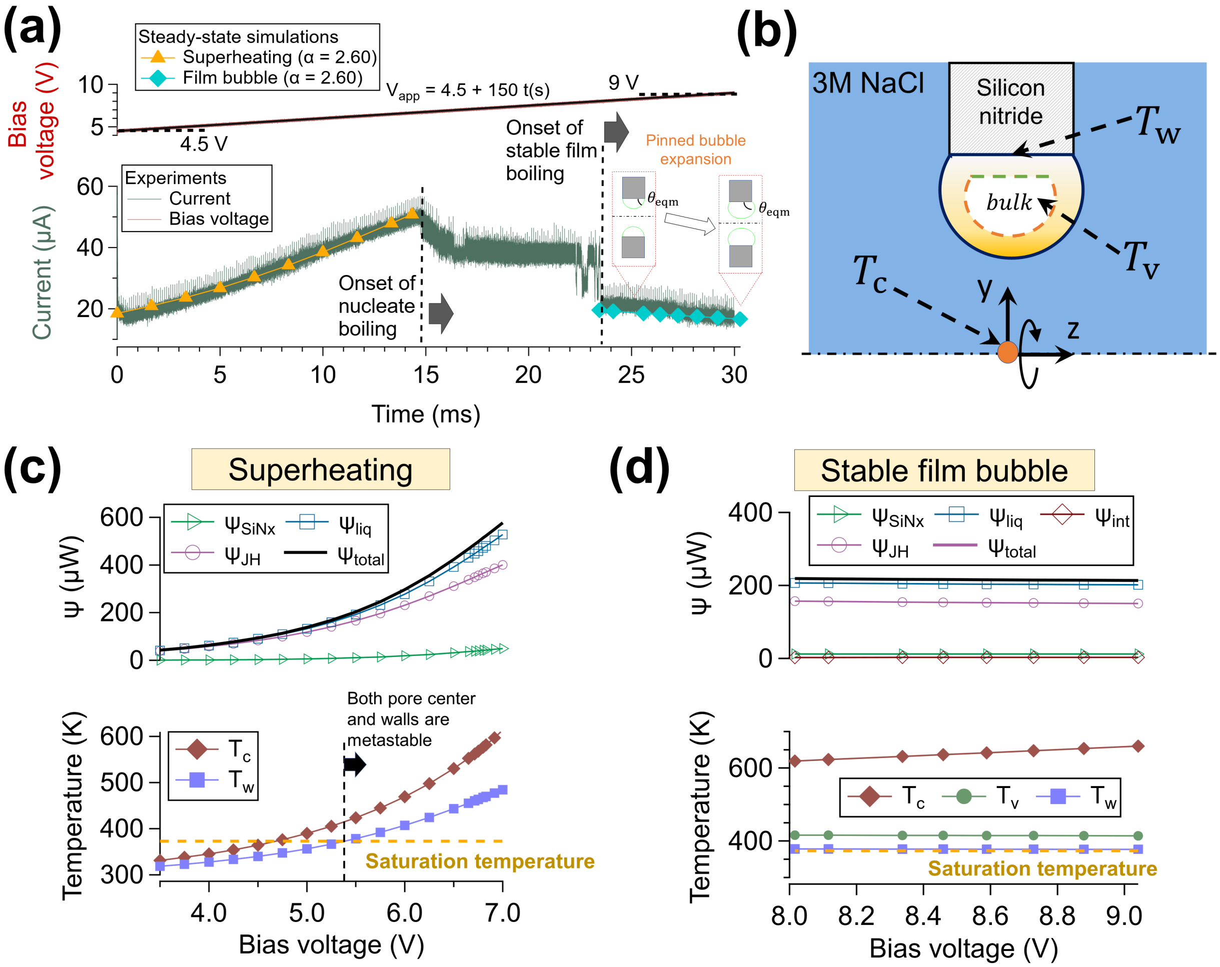


FIG. S4: (a) Variation of nanopore current with time as a ramp voltage is applied. (b) Schematic showing the definitions of pore center temperature $T_c$, pore surface temperature $T_w$, and vapor temperature inside film $T_v$, for nanopore boiling. Variations of nanopore temperatures and system dissipation during the (c) superheating and (d) stable film boiling phases of the nanopore boiling curve, respectively. These values were obtained from continuum simulations.

## S3. CHARACTERISTICS OF STABLE FILM BUBBLE

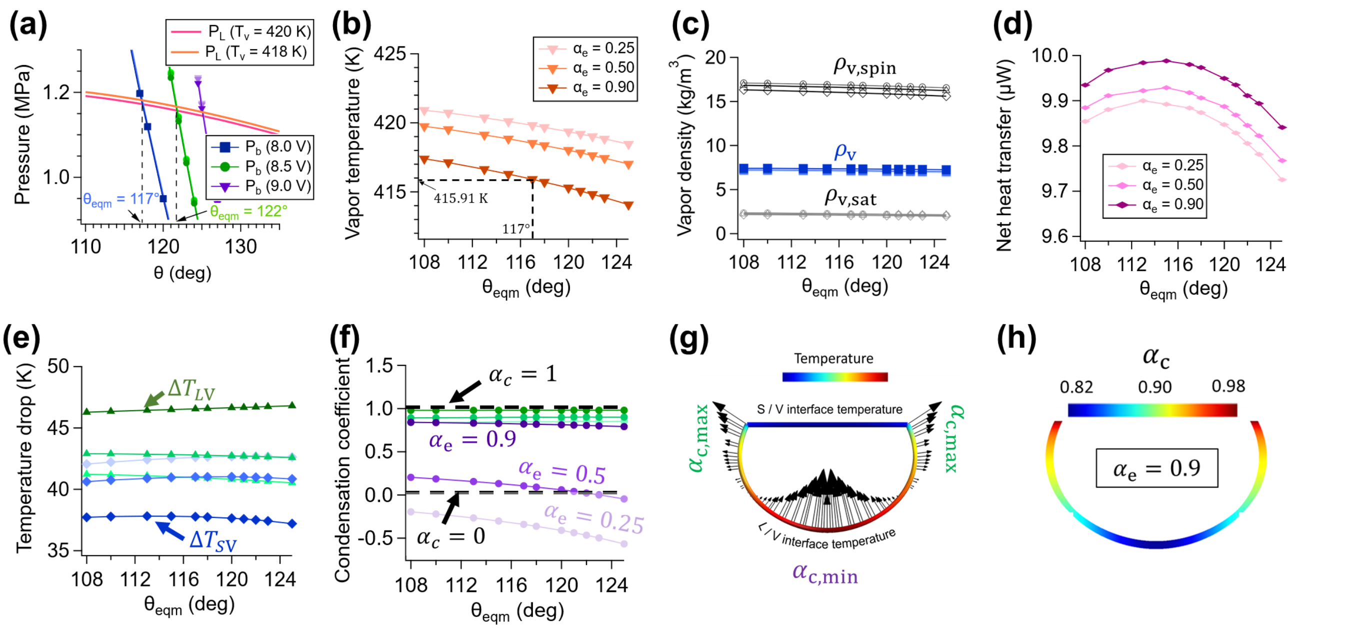


FIG. S5: (a) Film bubble shape at mechanical and dynamic thermal equilibrium during stable film boiling (SFB). The solid lines show the variation of Laplace pressure, while the lines with markers show the thermal steady state of the torus bubble [Eq. (6) in the main text]. (b) Vapor temperature. (c) Vapor density. (d) Total heat transferred through the bubble to the walls. (e) Average temperature drops $\Delta T_{\mathrm{LV}} = \bar{T}_{\mathrm{LV}} - T_{\mathrm{v}}$ and $\Delta T_{\mathrm{SV}} = T_{\mathrm{v}} - \bar{T}_{\mathrm{SV}}$ across the liquid–vapor and solid–vapor interfaces, respectively. (f) Variations of the minimum condensation coefficient (achieved at the bubble tip) and the maximum condensation coefficient (achieved at the bubble base) are shown by the purple and green traces. In each plot, the lightest shade corresponds to $\alpha_{\mathrm{e}} = 0.25$, the medium shade to $\alpha_{\mathrm{e}} = 0.5$, and the darkest shade to $\alpha_{\mathrm{e}} = 0.9$. (g) Temperature distributions on the LV and SV interfaces, with the vectors showing the mass influx and outflux on the LV surface. (h) Spatial variation or local self-organization of $\alpha_{\mathrm{c}}$ on the LV surface to ensure dynamic thermal equilibrium when $\alpha_{\mathrm{e}} = 0.9$ for the $\theta_{\mathrm{eqm}} = 117^{\circ}$ torus bubble at 8.02 V. Near the bubble tip, $\alpha_{\mathrm{c}}$ is at a minimum to accommodate the high heat fluxes from the liquid side. When $\alpha_{\mathrm{e}}$ is low (e.g., 0.25), the minimum $\alpha_{\mathrm{c}}$ becomes negative, which is unrealistic [Fig. S5(f)]. Hence, a stable film bubble is only possible for high $\alpha_{\mathrm{e}}$ (e.g., 0.9) in such extreme thermal environments.

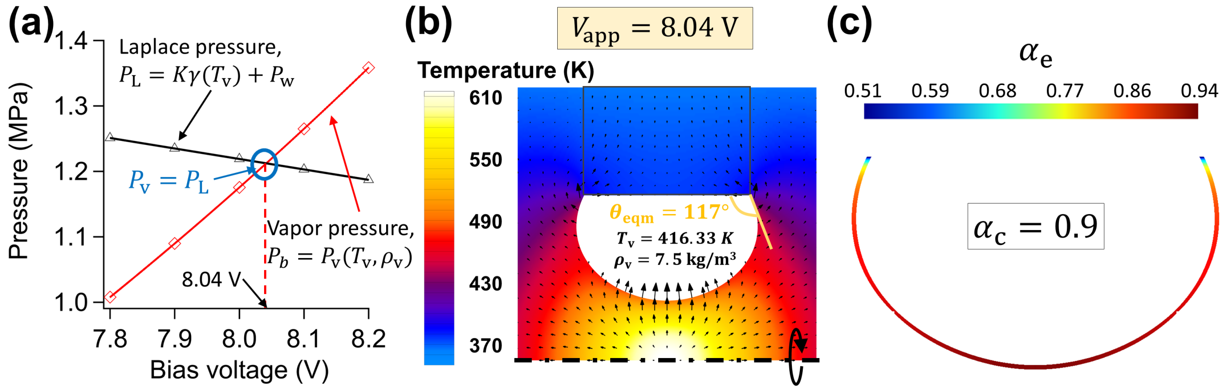


FIG. S6: (a) Film bubble at mechanical and dynamic thermal equilibrium for the $\theta = 117°$ bubble. The black line shows the variation of Laplace pressure, while the red line shows the vapor pressure within the thermally steady state torus bubble [Eq. (6) in the main text]. (b) Temperature profile around the $\theta_{\text{eqm}} = 117°$ nanopore torus bubble during stable film boiling at 8.04 V, and (c) variation of $\alpha_e$ on the LV interface. When $\alpha_c = 0.9$ is applied on the LV interface, $\alpha_e$ follows $\alpha_e = 1 - \frac{(1-\alpha_c)\rho_v}{\rho_{v,\text{sat}}}\sqrt{\frac{T_v}{T_{LV}}}$ to maintain the local conservation of fluxes.

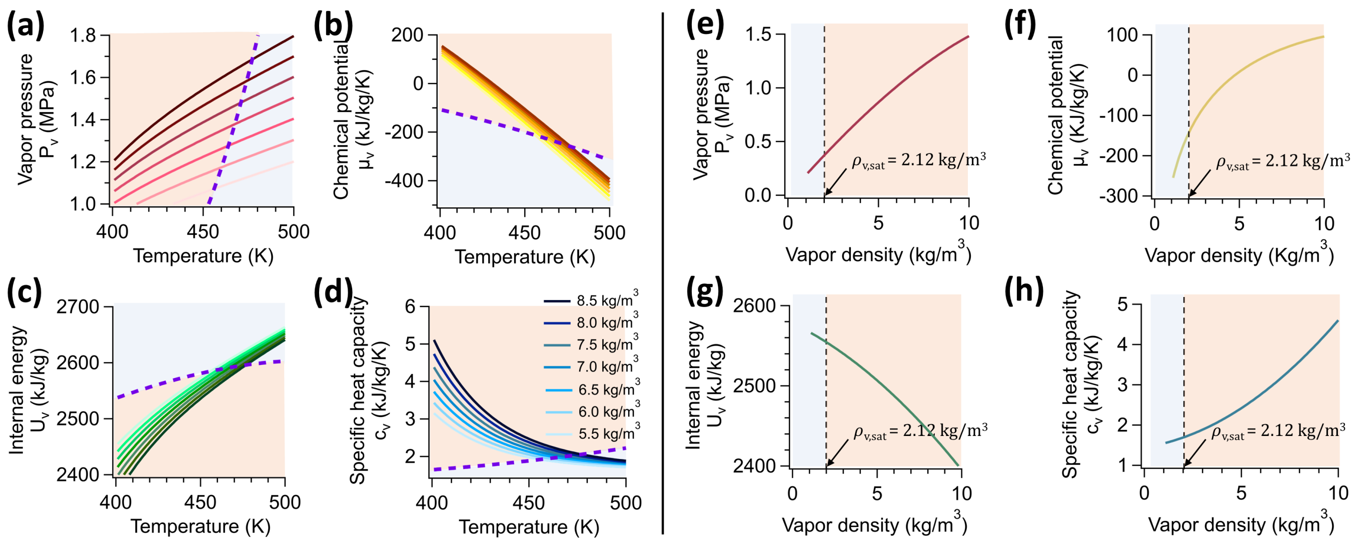


FIG. S7: Variation of (a) vapor pressure, (b) chemical potential, (c) internal energy, (d) isochoric specific heat energy with temperature, for different vapor densities. The lighter shades denote low density and darker shades denote high density as per the legend in (d). (e-h) show the variation of vapor pressure, chemical potential, internal energy, and isochoric specific heat energy with vapor density, keeping vapor temperature constant at $T_v = 416$ K. The metastable and single-phase vapor regions are shaded in orange and blue respectively. These properties were obtained using the gas equation given in the IAWPS-95 formulation for thermodynamic properties of water and steam [5].

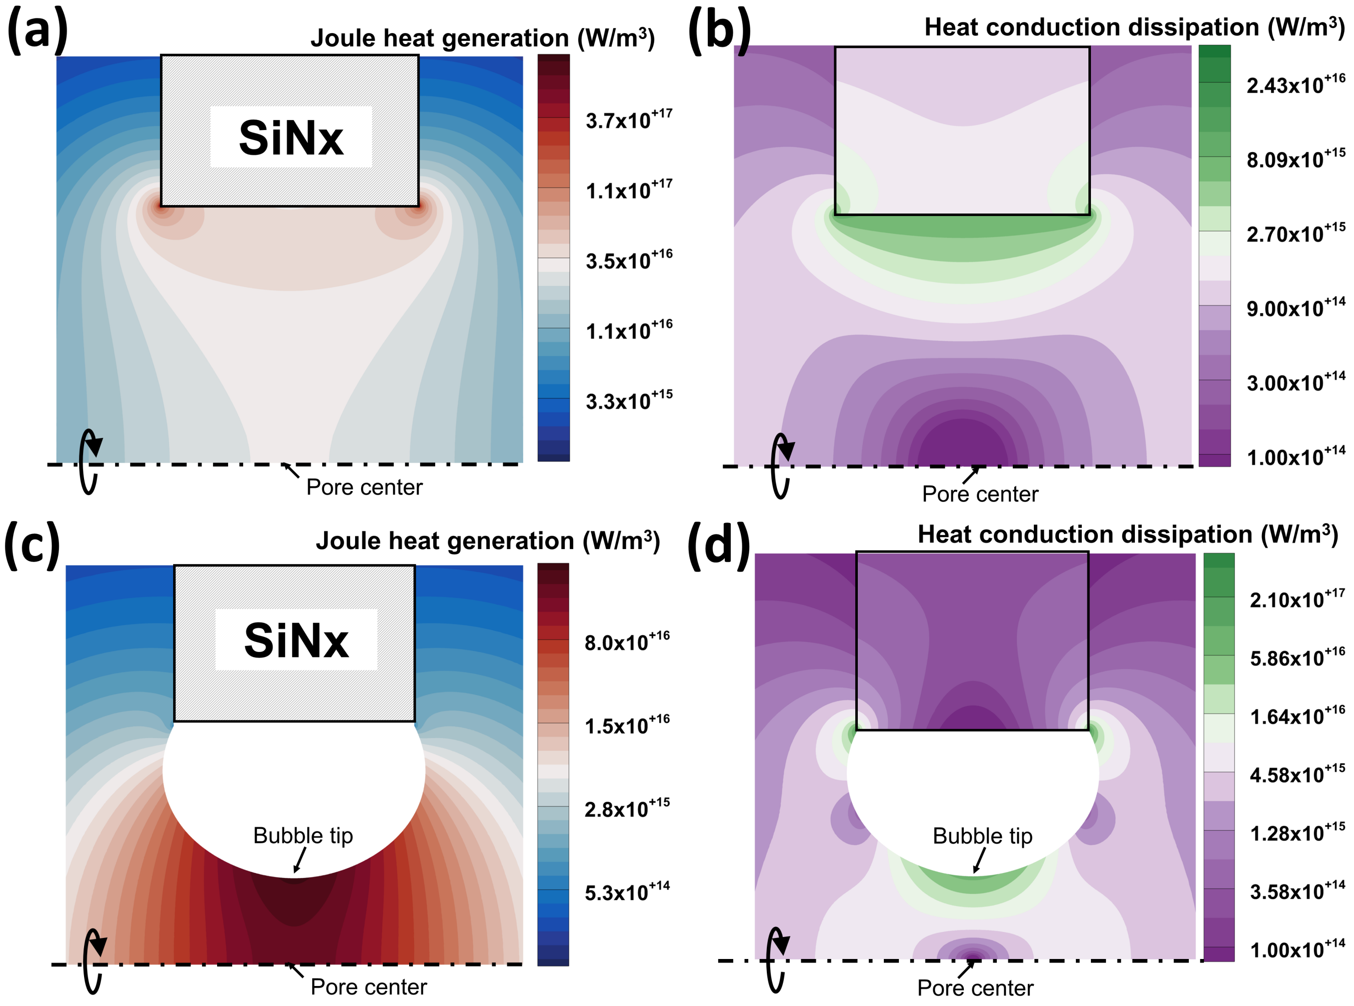


FIG. S8: (a) Joule heat density distribution and (b) heat conduction dissipation during superheating at 6.65 V. (c) Joule heat density distribution and (d) heat conduction dissipation around a $\theta_{\mathrm{eqm}} = 117°$ nanopore torus bubble during stable film boiling at 8.02 V. The colorbars are in exponential scale.

## S4. CHARACTERISTICS OF UNSTABLE FILM BUBBLE

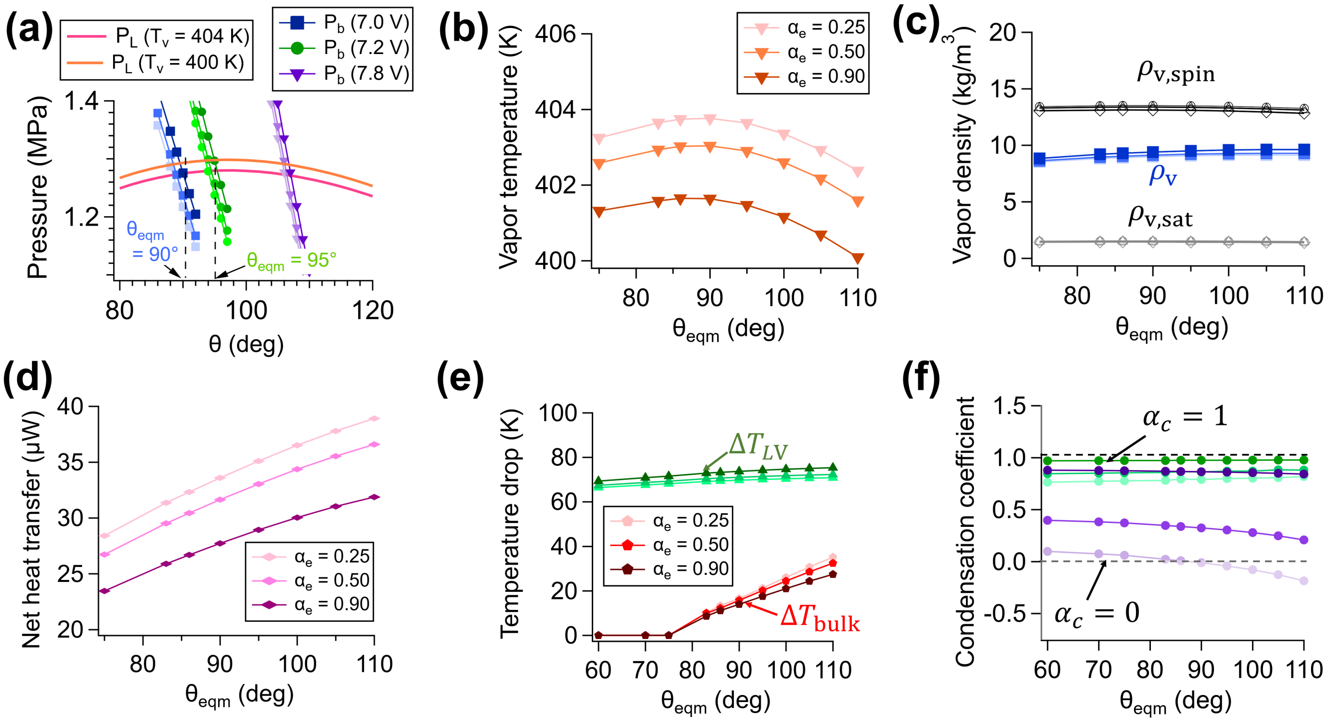


FIG. S9: (a) Film bubble shape at mechanical and dynamic thermal equilibrium during unstable film boiling (UFB). The solid lines show the variation of Laplace pressure while the lines with markers (blue, green, and purple) show the thermal steady state of the torus bubble [Eq. (6) in the main text]. The lightest shades of blue, green, and purple correspond to $\alpha_e = 0.25$, the medium shades to $\alpha_e = 0.5$, and the darkest shades to $\alpha_e = 0.9$. A similar shading sequence from light to dark for the three $\alpha_e$ values is adopted for the remaining subplots as well. It can be seen that the equilibrium bubble size $\theta_{eqm}$ is only slightly affected by the variation in $\alpha_e$. (b) Vapor temperature. (c) Vapor density. (d) Net heat transferred from liquid through the bubble to the walls. (e) Average temperature drops $\Delta T_{LV} = \bar{T}_{LV} - T_v$ and $\Delta T_{bulk}$ across the liquid–vapor interface and bulk vapor region, respectively. (f) Variations of the minimum condensation coefficient (achieved at the bubble tip) and the maximum condensation coefficient (achieved at the bubble base) are shown by the purple and green traces.

$\Delta T_{bulk}$ was solved for using a one-dimensional thermomass model that captures the diffusio-ballistic dynamics of heat transfer [6, 7]:

$$q_{net} = \frac{\sqrt{1+\zeta^2}-1}{\zeta} q_{max},$$

where $q_{max} = \bar{u}_v \rho_v c_v T_v$ and $\zeta = 2k_v \Delta T_{bulk}/(q_{max} h_{bulk,avg})$, with $h_{bulk,avg} = h_{avg} - \lambda$. Here, $k_v = \frac{1}{3}\rho_v c_v \lambda \bar{u}_v$ is the thermal conductivity, and $\bar{u}_v = 8k_B T_v/(\pi m)$ is the mean vapor velocity. $\Delta T_{bulk} = 0$ is taken for small bubbles ($\theta = 60°$ to $\theta = 75°$) when $h_{avg} < \lambda$.

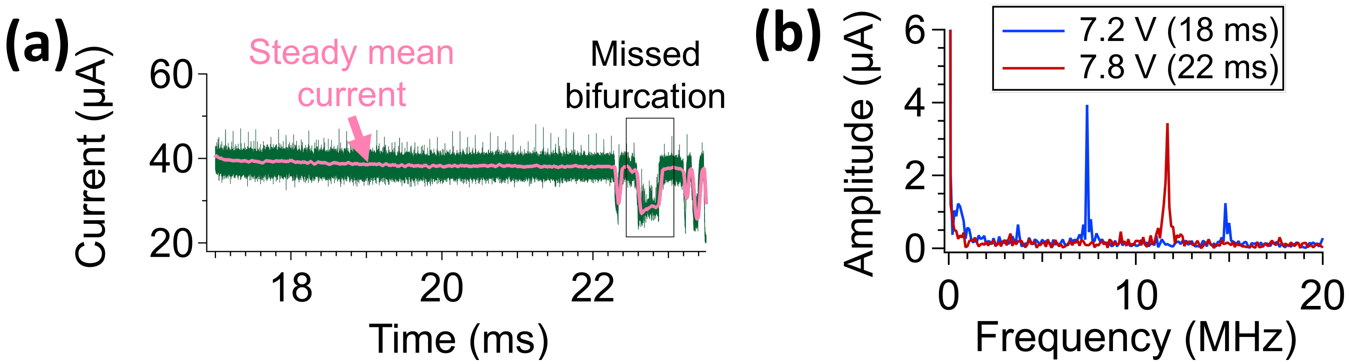


FIG. S10: (a) Mean current during the unstable film boiling (UFB) regime of the 199 nm pore boiling curve for the first voltage pulse P1 as shown in Fig. 4(e) in the main text. (b) Fast Fourier transform (FFT) of the nanopore current.

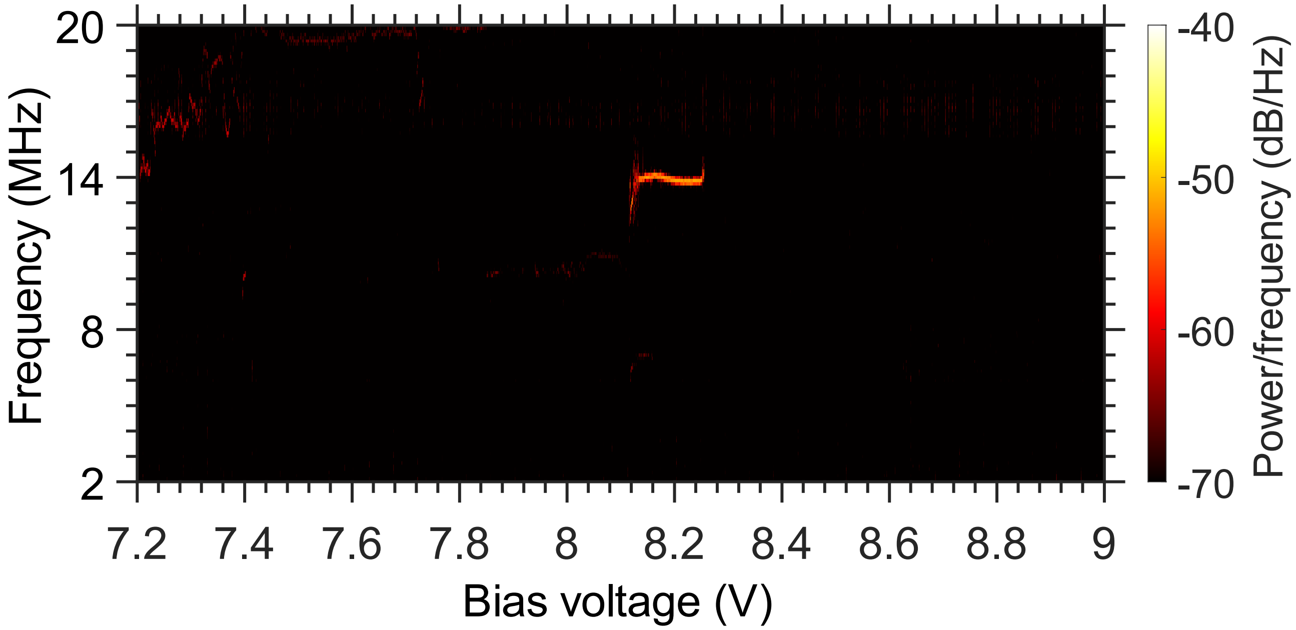


FIG. S11: Spectrogram of nanopore current during the UFB regime for the second voltage pulse P2 as shown in Fig. 4(e) in the main text.

## S5. SYSTEM DISSIPATION FUNCTION

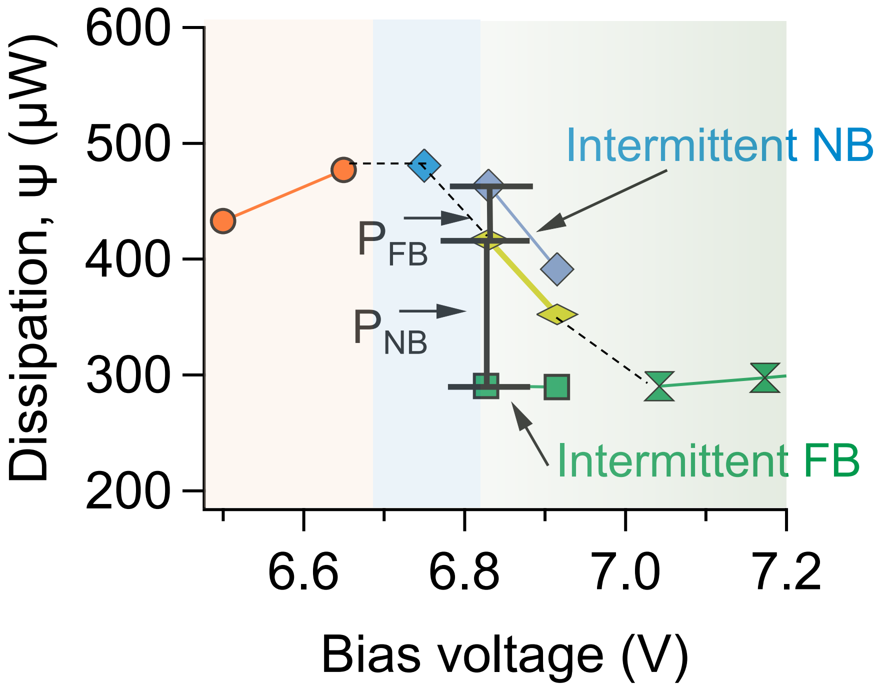


FIG. S12: Zoomed view of dissipation function near the first bifurcation point. The dissipation functions for the nucleate and film boiling are calculated for a given voltage. The net dissipation function is the weighted mean of the nucleate and film boiling taking account of their relative duration of prevalence as observed in experiments ($\Psi = \Psi_{\rm IFB}P_{\rm FB} + \Psi_{\rm INB}P_{\rm NB}$). Between $t = 15.333$ ms to $t = 15.733$ ms, when voltage varies linearly from 6.8 V to 6.86 V with a mean voltage of 6.83 V, $(P_{\rm FB}, P_{\rm NB}) = (0.27, 0.73)$ was observed. On the other hand, between $t = 15.900$ ms to $t = 16.300$ ms, when voltage varies linearly from 6.89 V to 6.95 V with a mean voltage of 6.92 V, $(P_{\rm FB}, P_{\rm NB}) = (0.38, 0.62)$, was observed. Film bubbles appear more frequently as the voltage is increased during intermittent film boiling.

The entropy generations for conduction heat transfer at the LV interface can be written as

$$\begin{aligned}\Psi_{\rm h,LV} &= \iint_{S_{\rm LV}} \frac{J_{\rm r,i}c_{\rm v}(T_{\rm LV}-T_{\rm v})^2}{T_{\rm v}}\,dS,\\ \Psi_{\rm h,SV} &= \iint_{S_{\rm SV}} \frac{J_{\rm r,w}c_{\rm v}(T_{\rm v}-T_{\rm SV})^2}{T_{\rm v}}\,dS,\end{aligned} \tag{S4}$$

where $J_{\rm r,i} = (1-\alpha_{\rm e})J_{\rm out} = (1-\alpha_{\rm e})\rho_{\rm v,sat}\sqrt{R_{\rm g}T_{\rm LV}/2\pi}$ and $J_{\rm r,w} = \rho_{\rm v}\sqrt{R_{\rm g}T_{\rm v}/2\pi}$ are the reflection fluxes on the LV and SV interface as shown in Figs. 2(d) and 2(c) in the main text. The entropy generation for evaporation/condensation mass transfer at the LV interface can be written as

$$\Psi_{\rm m,LV} = \iint_{S_{\rm LV}} \left[-\dot{m}T_{\rm v}\left(\frac{\mu_{\rm sat}}{T_{\rm LV}} - \frac{\mu_{\rm v}}{T_{\rm v}}\right)\right] dS, \tag{S5}$$

where $\dot{m}$ is the mass flux defined in Eq. (4) in the main text. $\mu_{\rm sat}$ is the chemical potential of the saturated vapor at $T_{\rm LV}$, and $\mu_{\rm v}$ is the chemical potential of the metastable vapor within the torus bubble at temperature $T_{\rm v}$ and density $\rho_{\rm v}$ [Figs. S5(b), S5(c), S9(b), and S9(c)], calculated using the IAWPS formulation [5]. $S_{\rm LV}$ and $S_{\rm SV}$ are the surface areas of the bubble interfaces as shown in Fig. S2 (right inset).

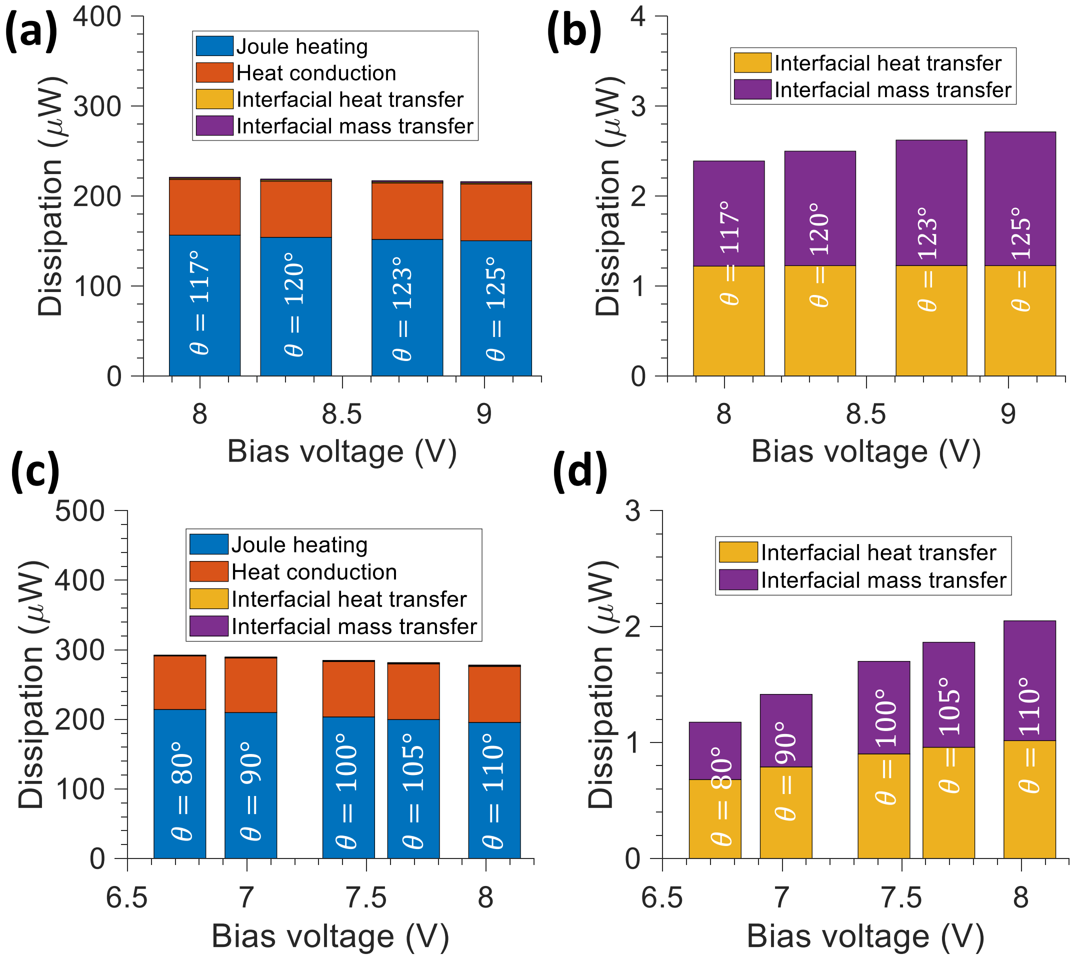


FIG. S13: Breakdown of dissipation function into individual contributions from liquid Joule heating, heat conduction in liquid and SiNx membrane, interfacial heat transfer on bubble interfaces, and interfacial mass transfer at the liquid–vapor interface for a stable film bubble [(a) and (b)] and for an unstable film bubble [(c) and (d)]. The evaporation accommodation coefficient is taken as $\alpha_e = 0.9$.

---


[1] E. V. Levine, M. M. Burns, and J. A. Golovchenko, Nanoscale Dynamics of Joule Heating and Bubble Nucleation in a Solid-State Nanopore, Phys. Rev. E **93**, 13124 (2016).

[2] S. Paul, W.-L. Hsu, M. Magnini, L. R. Mason, Y.-L. Ho, O. K. Matar, and H. Daiguji, Single-Bubble Dynamics in Nanopores: Transition between Homogeneous and Heterogeneous Nucleation, Phys. Rev. Res. **2**, 043400 (2020).

[3] D. J. E. Harvie, An Implicit Finite Volume Method for Arbitrary Transport Equations, ANZIAM J. **52**, 1126 (2012).

[4] C. T. Avedisian, The Homogeneous Nucleation Limits of Liquids, J. Phys. Chem. Ref. Data **14**, 695 (1985).

[5] W. Wagner and A. Pruß, The IAPWS Formulation 1995 for the Thermodynamic Properties of Ordinary Water Substance for General and Scientific Use, J. Phys. Chem. Ref. Data **31**, 387 (2002).

[6] A. Sellitto and V. A. Cimmelli, A Continuum Approach to Thermomass Theory, J. Heat Transf. **134**, 112402 (2012).

[7] Y. Guo and M. Wang, Phonon Hydrodynamics and Its Applications in Nanoscale Heat Transport, Phys. Rep. **595**, 1 (2015).
